# Supplementary material for: Hyperbolic Fracton Model, Subsystem Symmetry and Holography III: Extension to Generic Tessellations
Source: arXiv:2510.25994 source file (2026-04-15)
Supplement: Supplementary file 1 [file appendix.tex]

\section{Euclidean Fracton Models}
\subsection{Plaquette Ising Model}
The Plaquette Ising model can also be constructed using the inflation formalism. This offers another method to prove that the entropy of this model is subextensive, scaling with the boundary of the system. The inflation rule describing the model is:
\begin{align*}
\tau: \quad \sigma &\to \beta^4 \alpha^4\\
\alpha &\to \beta\alpha\beta \\
\beta &\to \beta
\end{align*}

Using the same reasoning as in the main text, the ground-state entropy of the PIM is: 
\begin{align*}
    S = k_B \log{2} \times \left(1 + \sum_{k=1}^{l} 4 \right) \\\\
    S = k_B \log{2} \times \left(1 + 4l \right)
\end{align*}

We get the residual ground-state entropy by dividing the entropy by the total number of spins and then taking the thermodynamic limit:
\begin{align*}
    \cfrac{S}{N_p} =  k_B \log{2} \times \left( \cfrac{1}{1 + \frac{4l^2}{1+4l}} \right) \\\\
    s = \lim_{l\to\infty} \cfrac{S}{N_p} \to 0.    
\end{align*}

And by dividing the entropy by the total number of spins on the boundary, then taking the thermodynamic limit we get:
\begin{align*}
    \cfrac{S}{N^l_{\alpha} + N^l_{\beta}} =  k_B \log{2} \times \left( \cfrac{1+4l}{4 + 4(2l-1)} \right) \\\\
    \lim_{l\to\infty} \cfrac{S}{N^l_{\alpha} + N^l_{\beta}} \to \frac{1}{2}k_B \log{2}.    
\end{align*}

This confirms that the entropy of the system scales with the boundary of the system rather than with its volume, therefore showing a sub-extensive ground-state degeneracy. 

\subsection{Hexagonal Tessellation}
The $\{6,3\}$ tessellation can be described by an inflation rule $\tau$, as demonstrated in the main text for the hyperbolic $\{p,3\}$ tessellations:
\begin{align*}
\tau: \quad \sigma &\to \beta^6 \\
\beta &\to \gamma^{1/2}\beta\gamma^{1/2} \\   
\gamma &\to \gamma
\end{align*}

The connectivity of the lattice is such that for layers $l>1$ the number of constraints is greater than the number of spins, thus resulting in a four-fold ground state degeneracy. The degeneracy arises from the orientation of the central spin the initial layer's orientation as we illustrate in Fig.~\ref{fig:6,3-tessellation}.
\begin{figure}
    \centering
    \includegraphics[width=1\linewidth]{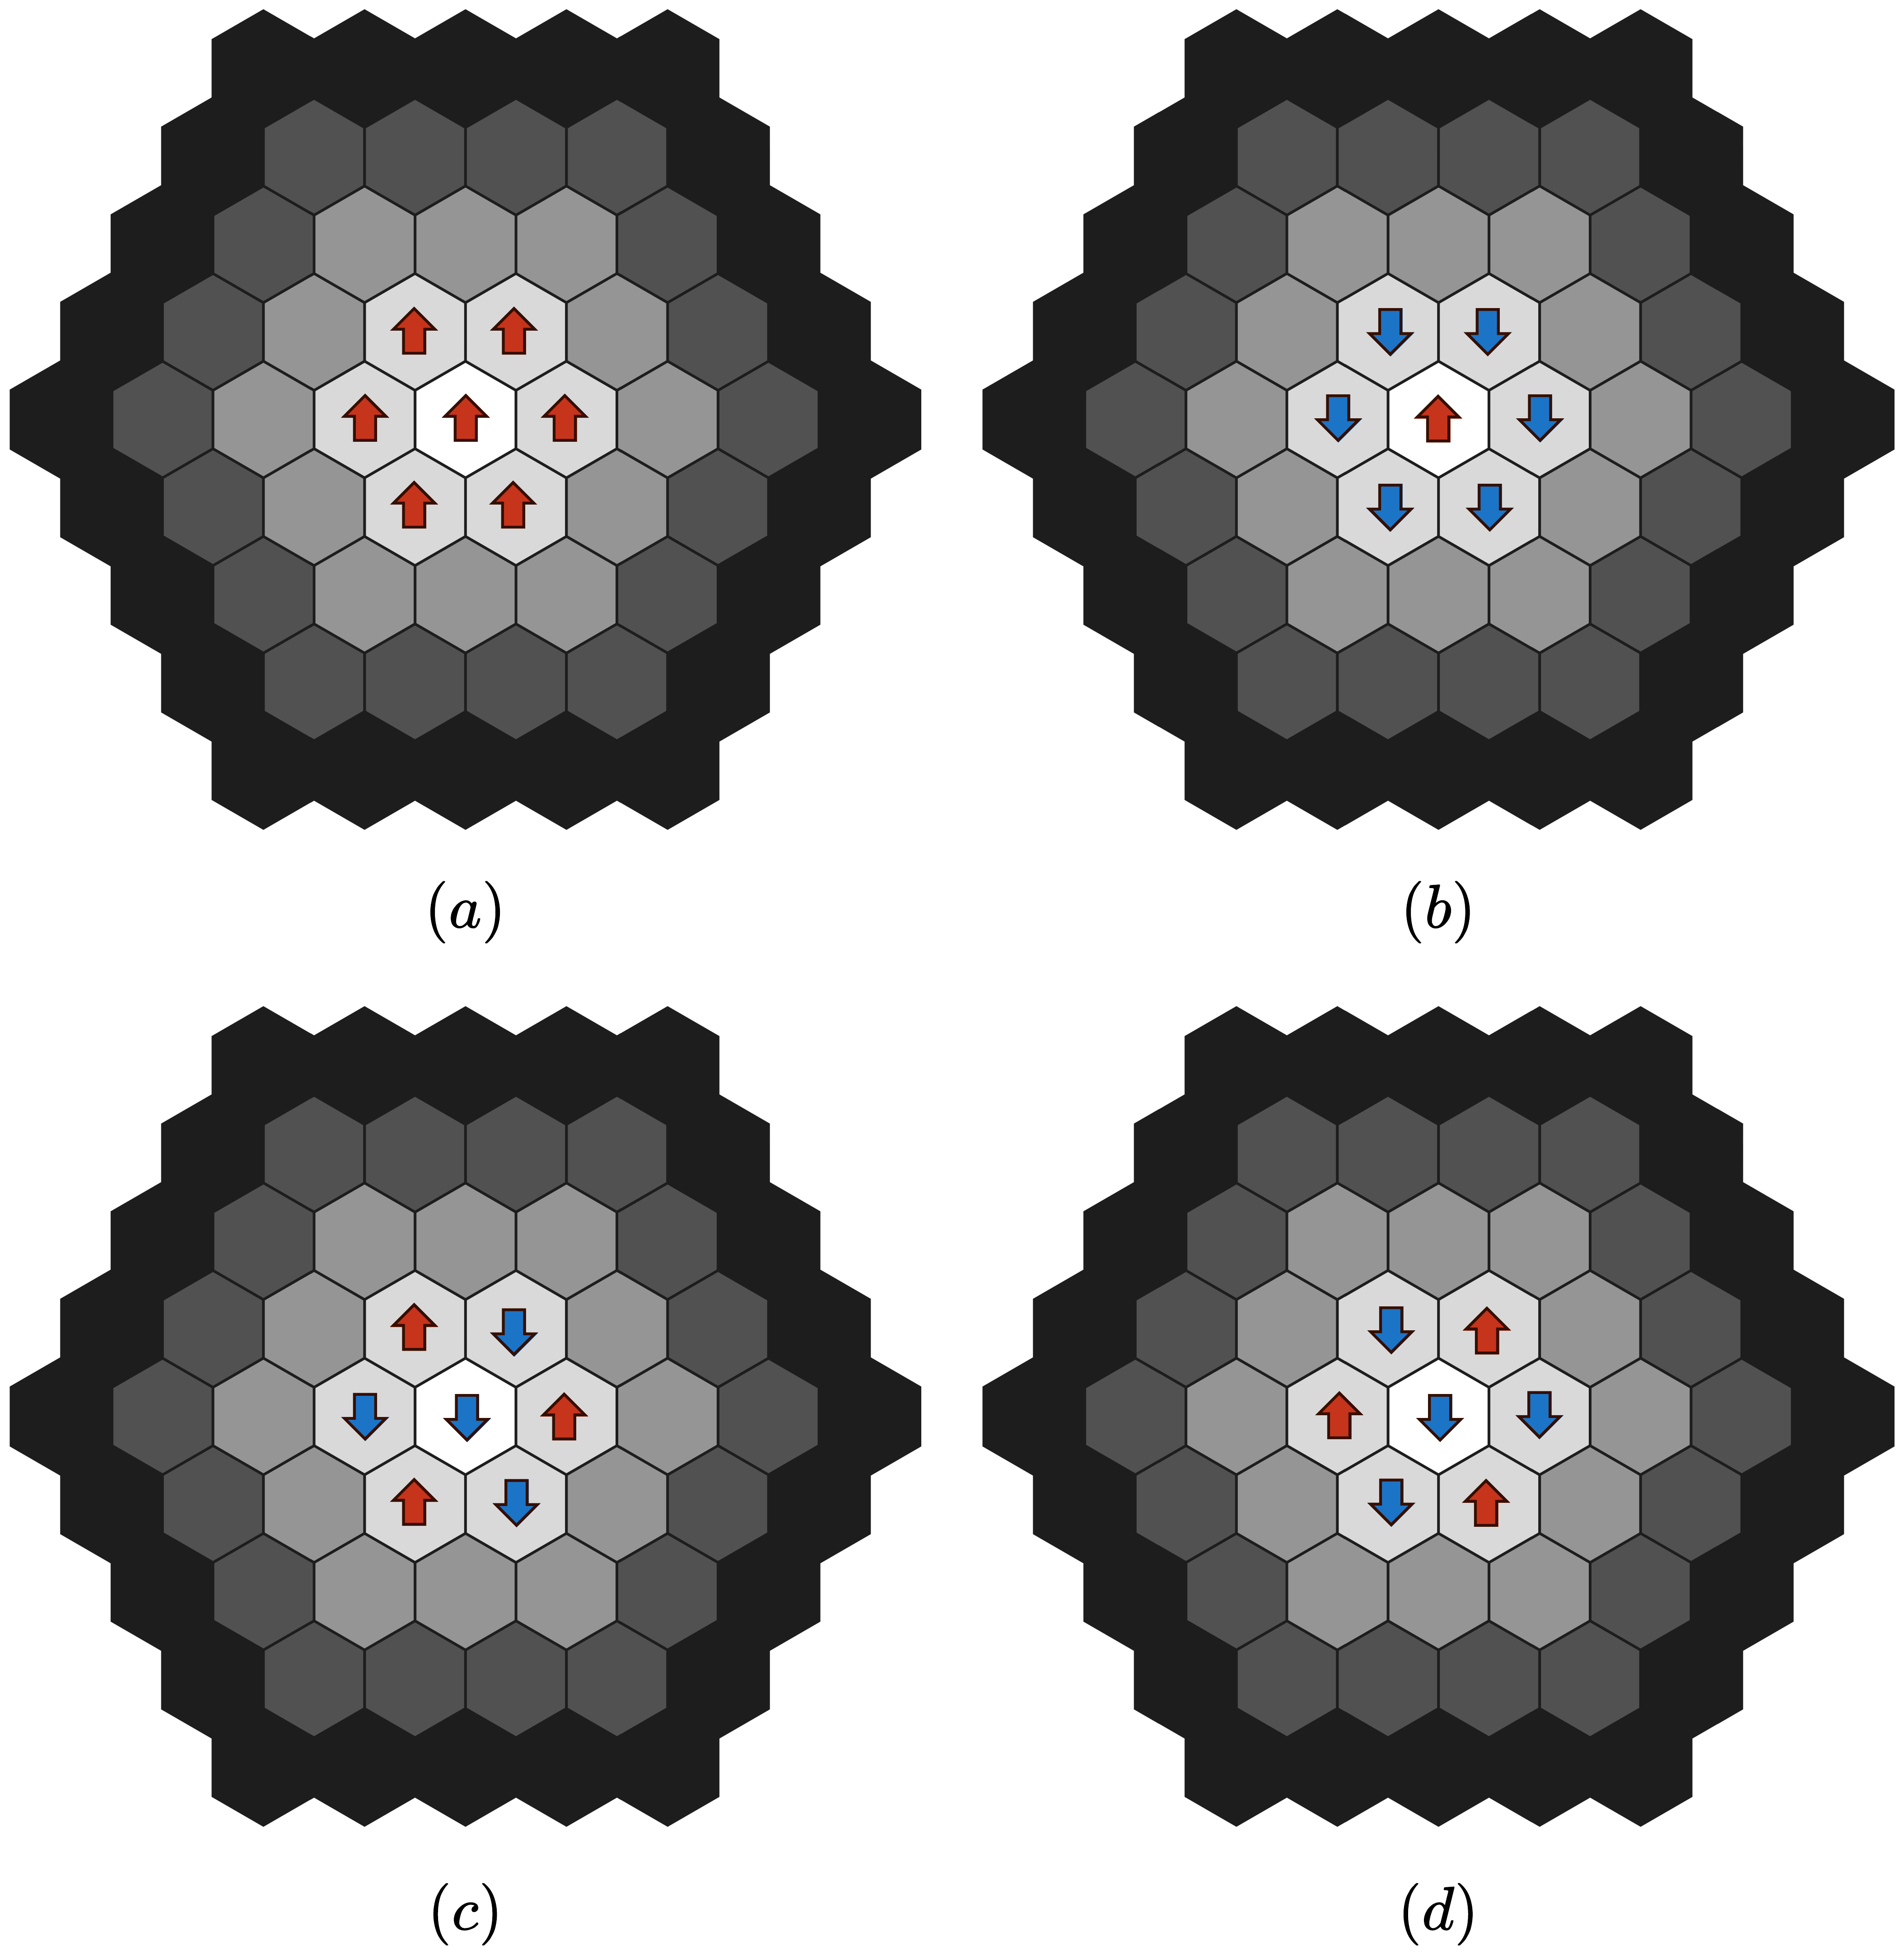}
    \caption{The four ground states of the hexagonal tessellation. $(a)$ and $(b)$ are ground states where the central spin chosen to be up, while $(c)$ and $(d)$ correspond to the spin down choice. }
    \label{fig:6,3-tessellation}
\end{figure}
\subsection{Triangular Tessellation}

The $\{3,6\}$ tessellation is described by the inflation rule $\tau$:
\begin{align*}
\tau: \quad \sigma &\to \beta^3 \alpha^3\\
\alpha &\to \alpha\beta\alpha \\
\beta &\to \alpha^{-1}  
\end{align*}

The ground-state entropy is:
\begin{align*}
    S = k_B \log{2} \times \left(1 + 3l(l+2) \right)
\end{align*}

Surprisingly and in contrast to the square tessellation, the residual entropy of the system on this lattice is nonzero and is given by:
\begin{align*}
    \cfrac{S}{N_p} =  k_B \log{2} \times \left( \cfrac{1 + 3l(l+2)}{1 + 6l(l+1)} \right) \\\\
    s = \lim_{l\to\infty} \cfrac{S}{N_p} \to \frac{1}{2}k_B \log{2}.    
\end{align*}

Upon closer inspection of the model, the extensive entropy can be understood geometrically. With six triangles meeting at a vertex the system is under-constrained and allows for fluctuations of the spins. These fluctuations manifest as loops of spin flips that preserve the ground-state (and also appear for the hyperbolic $\{3,q\}$ tessellations), as illustrated in Fig.~\ref{fig:3,6-tessellation}.
\begin{figure}
    \centering
    \includegraphics[width=1\linewidth]{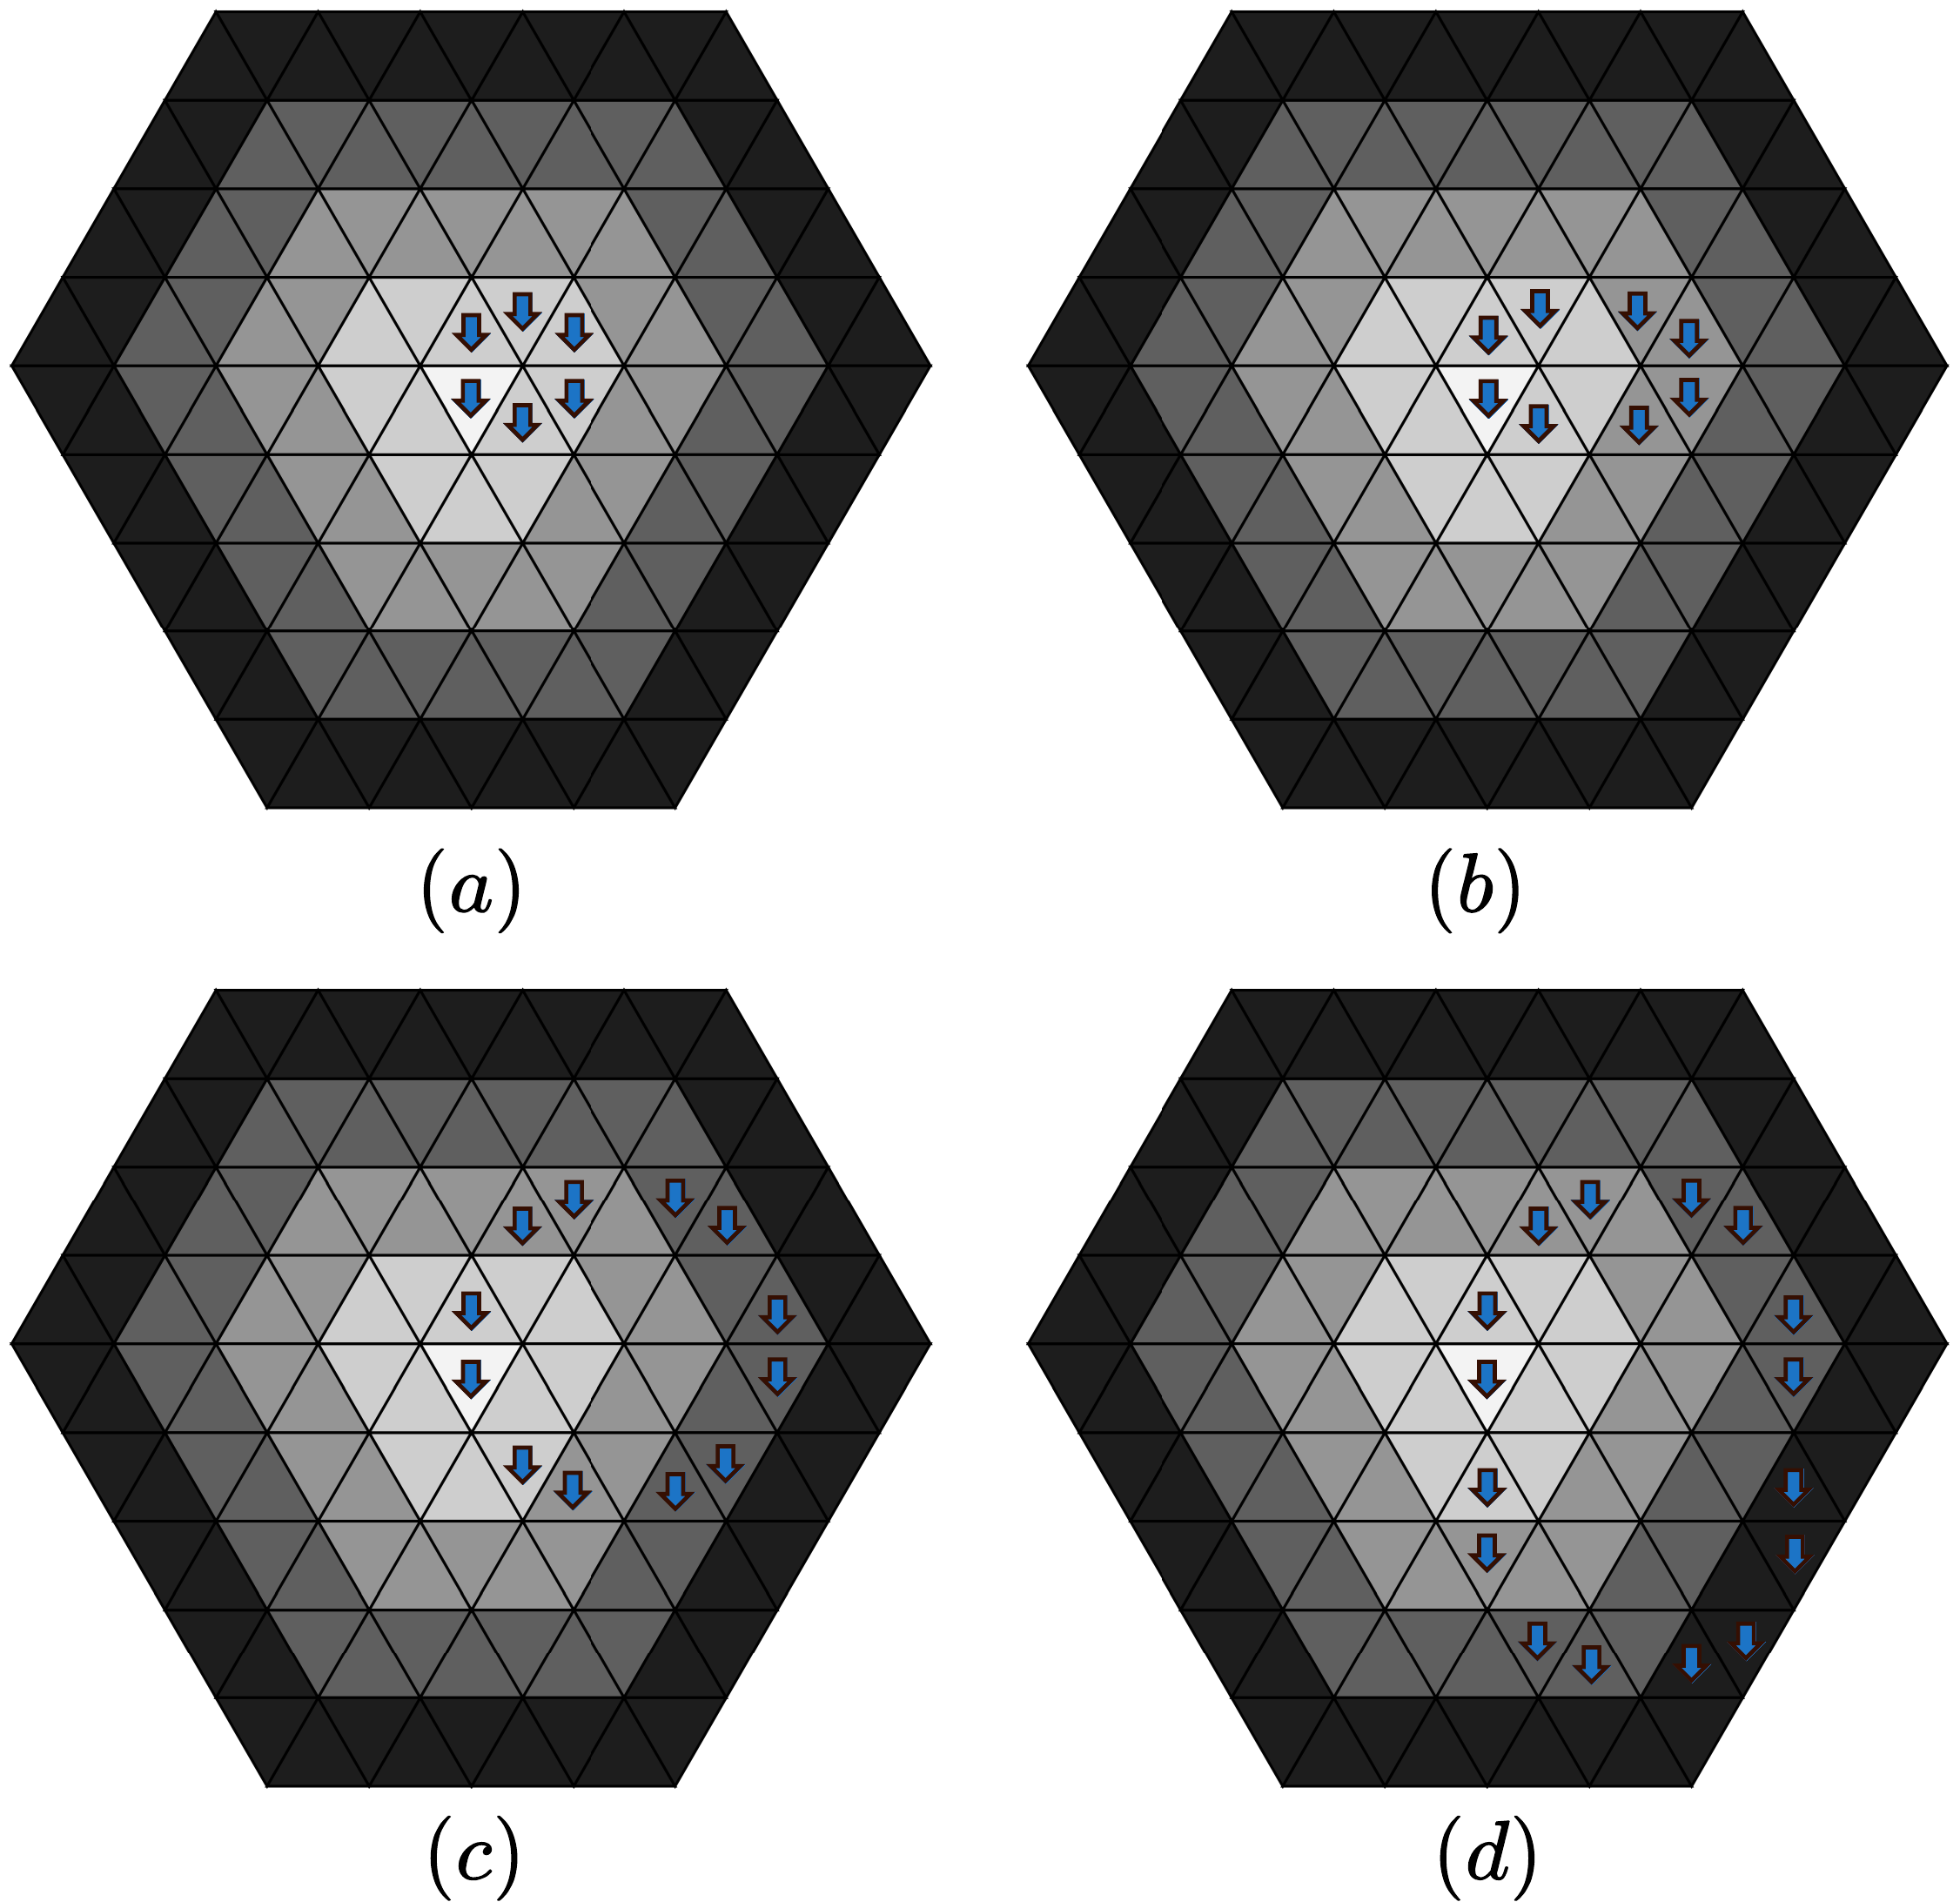}
    \caption{Example of loops of spin flips that can be formed on the $\{3,6\}$ tessellation, contributing to the extensive ground-state degeneracy.}
    \label{fig:3,6-tessellation}
\end{figure}
